# Supplementary material for: ELUDE: Generating interpretable explanations via a decomposition into labelled and unlabelled features
Source: arXiv:2206.07690 source file (2022-06-16)
Supplement: Supplementary file 1 [file CAM_ade_supp.tex]

\begin{tabular}{r ccc}
\begin{tabular}{r}
\texttt{shopping}\\ \texttt{dining} 
\end{tabular} & \raisebox{-0.5\height}{\includegraphics[scale=0.185]{figs/CAM_ade20k/heatmap_pairs/0.png}} & \raisebox{-0.5\height}{\includegraphics[scale=0.185]{figs/CAM_ade20k/heatmap_pairs/1.png}} & \raisebox{-0.5\height}{\includegraphics[scale=0.185]{figs/CAM_ade20k/heatmap_pairs/2.png}} \\ 
%\begin{tabular}{r}
%\texttt{workplace}
%\end{tabular}
%& \raisebox{-0.5\height}{\includegraphics[scale=0.185]{figs/CAM_ade20k/heatmap_pairs/3.png}} & \raisebox{-0.5\height}{\includegraphics[scale=0.185]{figs/CAM_ade20k/heatmap_pairs/4.png}} & \raisebox{-0.5\height}{\includegraphics[scale=0.185]{figs/CAM_ade20k/heatmap_pairs/5.png}} \\
\texttt{home-hotel}
& \raisebox{-0.5\height}{\includegraphics[scale=0.185]{figs/CAM_ade20k/heatmap_pairs/6.png}} & \raisebox{-0.5\height}{\includegraphics[scale=0.185]{figs/CAM_ade20k/heatmap_pairs/7.png}} & \raisebox{-0.5\height}{\includegraphics[scale=0.185]{figs/CAM_ade20k/heatmap_pairs/8.png}} \\ 
\begin{tabular} {r}\texttt{indoor}\\\texttt{transpor-}\\\texttt{tation}\end{tabular} 
& \raisebox{-0.5\height}{\includegraphics[scale=0.185]{figs/CAM_ade20k/heatmap_pairs/9.png}} & \raisebox{-0.5\height}{\includegraphics[scale=0.185]{figs/CAM_ade20k/heatmap_pairs/10.png}} & \raisebox{-0.5\height}{\includegraphics[scale=0.185]{figs/CAM_ade20k/heatmap_pairs/11.png}} \\ 
%\begin{tabular}{r}\texttt{indoor sports/}\\\texttt{leisure}\end{tabular}
%& \raisebox{-0.5\height}{\includegraphics[scale=0.185]{figs/CAM_ade20k/heatmap_pairs/12.png}} & \raisebox{-0.5\height}{\includegraphics[scale=0.185]{figs/CAM_ade20k/heatmap_pairs/13.png}} & \raisebox{-0.5\height}{\includegraphics[scale=0.185]{figs/CAM_ade20k/heatmap_pairs/14.png}} \\ 
%\begin{tabular}{r}\texttt{indoor}\\\texttt{cultural}\end{tabular}
%& \raisebox{-0.5\height}{\includegraphics[scale=0.185]{figs/CAM_ade20k/heatmap_pairs/15.png}} & \raisebox{-0.5\height}{\includegraphics[scale=0.185]{figs/CAM_ade20k/heatmap_pairs/16.png}} & \raisebox{-0.5\height}{\includegraphics[scale=0.185]{figs/CAM_ade20k/heatmap_pairs/17.png}} \\ 
%\begin{tabular}{r}\texttt{water/}\\\texttt{ice/ snow}\end{tabular}
%& \raisebox{-0.5\height}{\includegraphics[scale=0.185]{figs/CAM_ade20k/heatmap_pairs/18.png}} & \raisebox{-0.5\height}{\includegraphics[scale=0.185]{figs/CAM_ade20k/heatmap_pairs/19.png}} & \raisebox{-0.5\height}{\includegraphics[scale=0.185]{figs/CAM_ade20k/heatmap_pairs/20.png}} \\ 
\begin{tabular}{r}\texttt{mountains}\\\texttt{desert}\\\texttt{sky}\end{tabular}
& \raisebox{-0.5\height}{\includegraphics[scale=0.185]{figs/CAM_ade20k/heatmap_pairs/21.png}} & \raisebox{-0.5\height}{\includegraphics[scale=0.185]{figs/CAM_ade20k/heatmap_pairs/22.png}} & \raisebox{-0.5\height}{\includegraphics[scale=0.185]{figs/CAM_ade20k/heatmap_pairs/23.png}} \\ 
\begin{tabular}{r}\texttt{forest}\\\texttt{field}\\\texttt{jungle}\end{tabular}
& \raisebox{-0.5\height}{\includegraphics[scale=0.185]{figs/CAM_ade20k/heatmap_pairs/24.png}} & \raisebox{-0.5\height}{\includegraphics[scale=0.185]{figs/CAM_ade20k/heatmap_pairs/25.png}} & \raisebox{-0.5\height}{\includegraphics[scale=0.185]{figs/CAM_ade20k/heatmap_pairs/26.png}} \\ 
\begin{tabular}{r}\texttt{outdoor}\\\texttt{manmade}\\\texttt{elements}\end{tabular}
& \raisebox{-0.5\height}{\includegraphics[scale=0.185]{figs/CAM_ade20k/heatmap_pairs/27.png}} & \raisebox{-0.5\height}{\includegraphics[scale=0.185]{figs/CAM_ade20k/heatmap_pairs/28.png}} & \raisebox{-0.5\height}{\includegraphics[scale=0.185]{figs/CAM_ade20k/heatmap_pairs/29.png}} \\ 
%\begin{tabular}{r}
%\texttt{outdoor}\\
%\texttt{transportation}
%\end{tabular}
%& \raisebox{-0.5\height}{\includegraphics[scale=0.185]{figs/CAM_ade20k/heatmap_pairs/30.png}} & \raisebox{-0.5\height}{\includegraphics[scale=0.185]{figs/CAM_ade20k/heatmap_pairs/31.png}} & \raisebox{-0.5\height}{\includegraphics[scale=0.185]{figs/CAM_ade20k/heatmap_pairs/32.png}} \\ 
\begin{tabular}{r}\texttt{cultural}\\\texttt{historical}\end{tabular}
& \raisebox{-0.5\height}{\includegraphics[scale=0.185]{figs/CAM_ade20k/heatmap_pairs/33.png}} & \raisebox{-0.5\height}{\includegraphics[scale=0.185]{figs/CAM_ade20k/heatmap_pairs/34.png}} & \raisebox{-0.5\height}{\includegraphics[scale=0.185]{figs/CAM_ade20k/heatmap_pairs/35.png}} \\ 
\begin{tabular}{r}\texttt{outdoor}\\\texttt{sportsfie-}\\\texttt{lds parks} \end{tabular}
& \raisebox{-0.5\height}{\includegraphics[scale=0.185]{figs/CAM_ade20k/heatmap_pairs/36.png}} & \raisebox{-0.5\height}{\includegraphics[scale=0.185]{figs/CAM_ade20k/heatmap_pairs/37.png}} & \raisebox{-0.5\height}{\includegraphics[scale=0.185]{figs/CAM_ade20k/heatmap_pairs/38.png}} \\ 
\begin{tabular}{r}\texttt{industrial}\\\texttt{constru-}\\\texttt{ction}\end{tabular}
& \raisebox{-0.5\height}{\includegraphics[scale=0.185]{figs/CAM_ade20k/heatmap_pairs/39.png}} & \raisebox{-0.5\height}{\includegraphics[scale=0.185]{figs/CAM_ade20k/heatmap_pairs/40.png}} & \raisebox{-0.5\height}{\includegraphics[scale=0.185]{figs/CAM_ade20k/heatmap_pairs/41.png}} \\ 
\begin{tabular}{r}\texttt{cabins}\\\texttt{gardens}\\\texttt{farms}\end{tabular}
& \raisebox{-0.5\height}{\includegraphics[scale=0.185]{figs/CAM_ade20k/heatmap_pairs/42.png}} & \raisebox{-0.5\height}{\includegraphics[scale=0.185]{figs/CAM_ade20k/heatmap_pairs/43.png}} & \raisebox{-0.5\height}{\includegraphics[scale=0.185]{figs/CAM_ade20k/heatmap_pairs/44.png}} \\ 
%\begin{tabular}{r}\texttt{buildings/}\\\texttt{towns}\end{tabular}
%& \raisebox{-0.5\height}{\includegraphics[scale=0.185]{figs/CAM_ade20k/heatmap_pairs/45.png}} & \raisebox{-0.5\height}{\includegraphics[scale=0.185]{figs/CAM_ade20k/heatmap_pairs/46.png}} & \raisebox{-0.5\height}{\includegraphics[scale=0.185]{figs/CAM_ade20k/heatmap_pairs/47.png}} \\ 
\end{tabular}
